# Supplementary material for: First Measurement of Charged Current Muon Neutrino-Induced $K^+$ Production on Argon using the MicroBooNE Detector
Source: arXiv:2503.00291 ancillary file (2025-11-13)
Supplement: Supplementary file 1 [file MicroBooNE_Kaon_production_Supplemental_Material_v2.pdf]

# FIRST MEASUREMENT OF CHARGED CURRENT MUON NEUTRINO-INDUCED $K^+$ PRODUCTION ON ARGON USING THE MICROBOONE DETECTOR

## I. DATA/MC COMPARISON FOR SIDEBANDS

This section shows data/MC comparisons for different kinematic variables studied in this analysis. The data used for the comparison is equivalent to a total of  $6.88 \times 10^{20}$  POT (MicroBooNE Run 1-3 datasets).

A near and far sideband region were defined based on a 2D plot of the BDT score vs. daughter track length, as shown in Figure 1. The near and far sideband data/MC comparison shows good agreement (within the statistical uncertainty, see Figure 2 and 3) for kinematic variables studied during the development of this analysis. The agreement with data shows that the background predictions from the MC can be used in the single-bin flux-integrated cross-section measurement without the need to implement a background constraint. The  $\chi^2$  value for each distribution in Figures 2 and 3 were calculated using Pearson's  $\chi^2$  test, only considering statistical uncertainty.

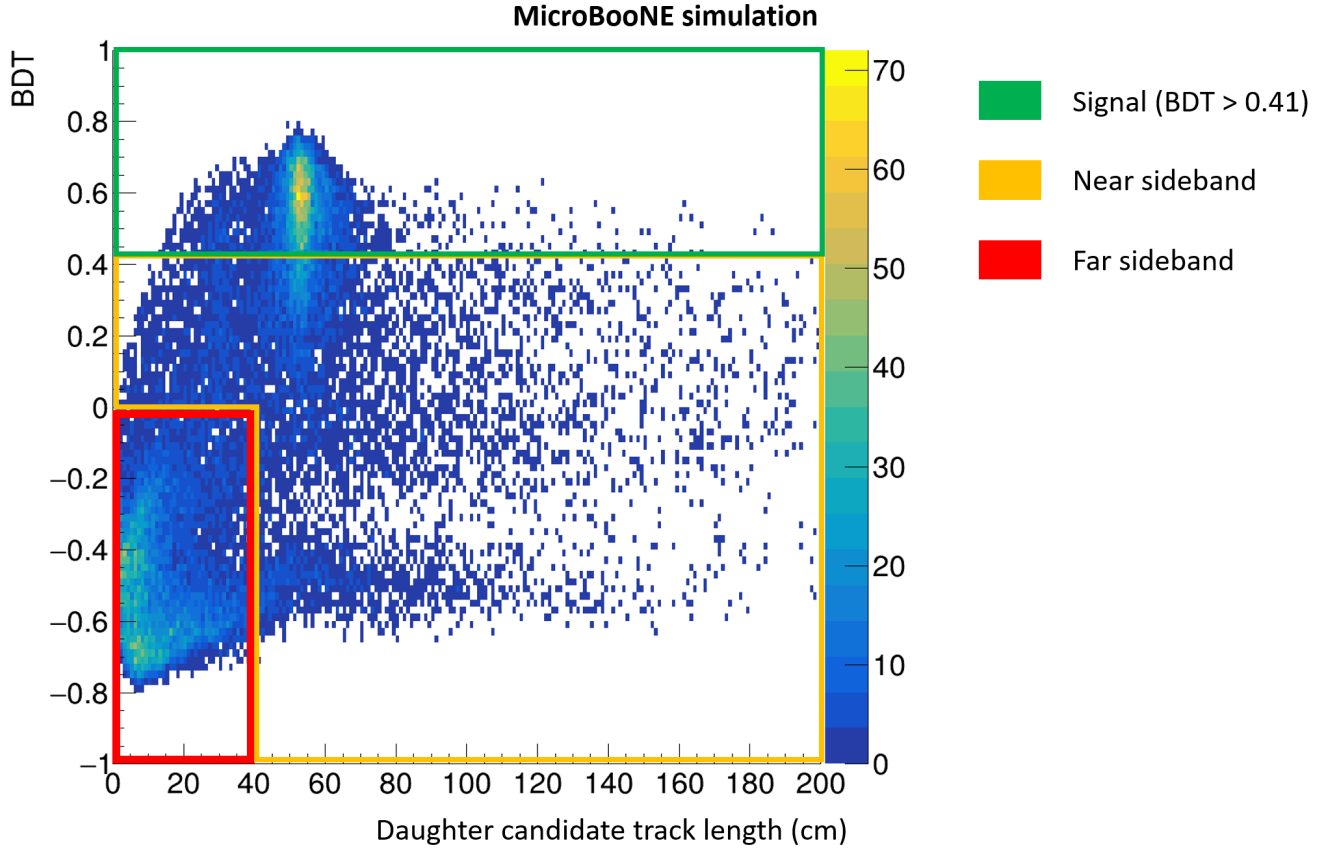

Figure 1: Sideband regions used in this analysis. Signal region (BDT > 0.41, green region), near sideband (yellow region), and far sideband (red region).

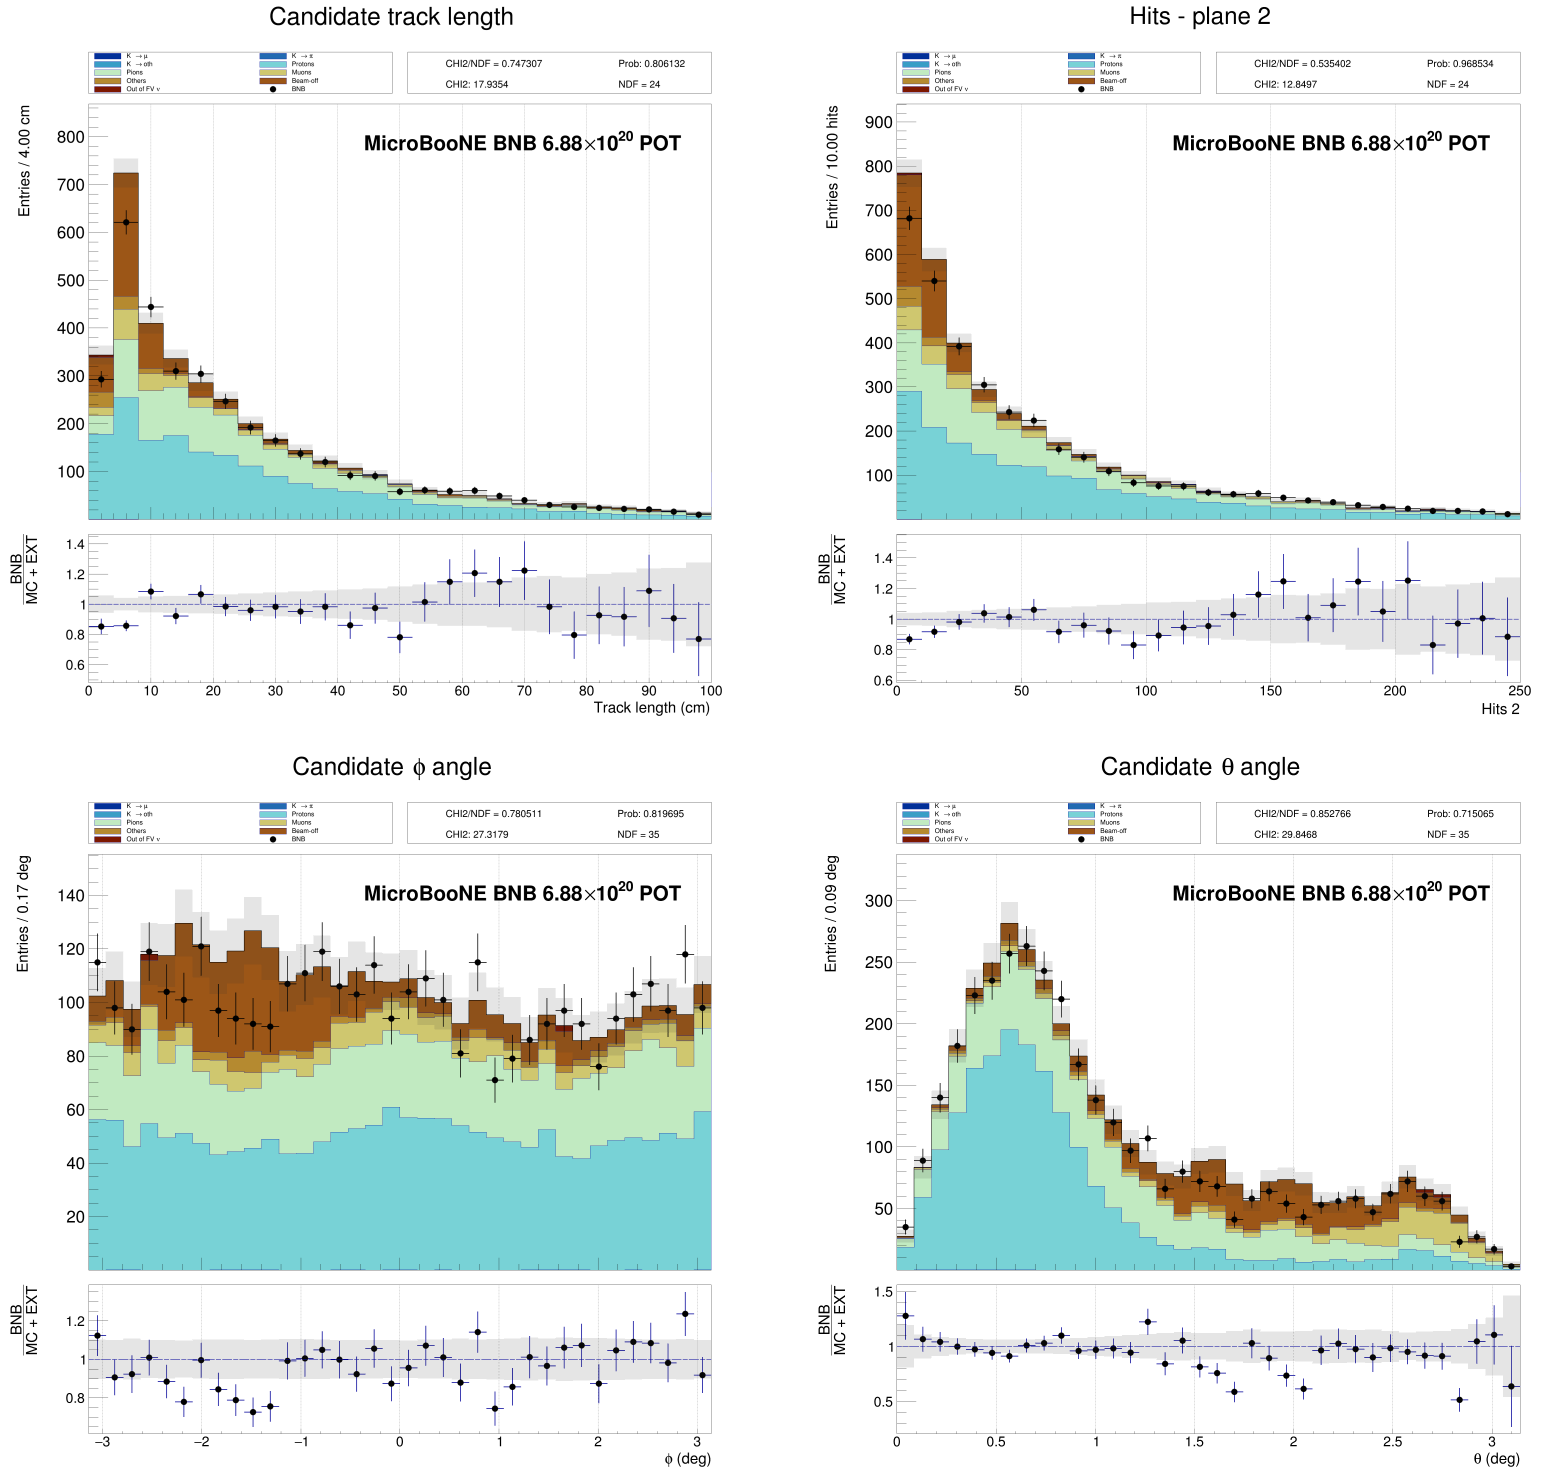

Figure 2: Far sideband data/MC comparisons for track length,  $\phi$ ,  $\theta$  angles, number of hits on collection plane (plane 2).

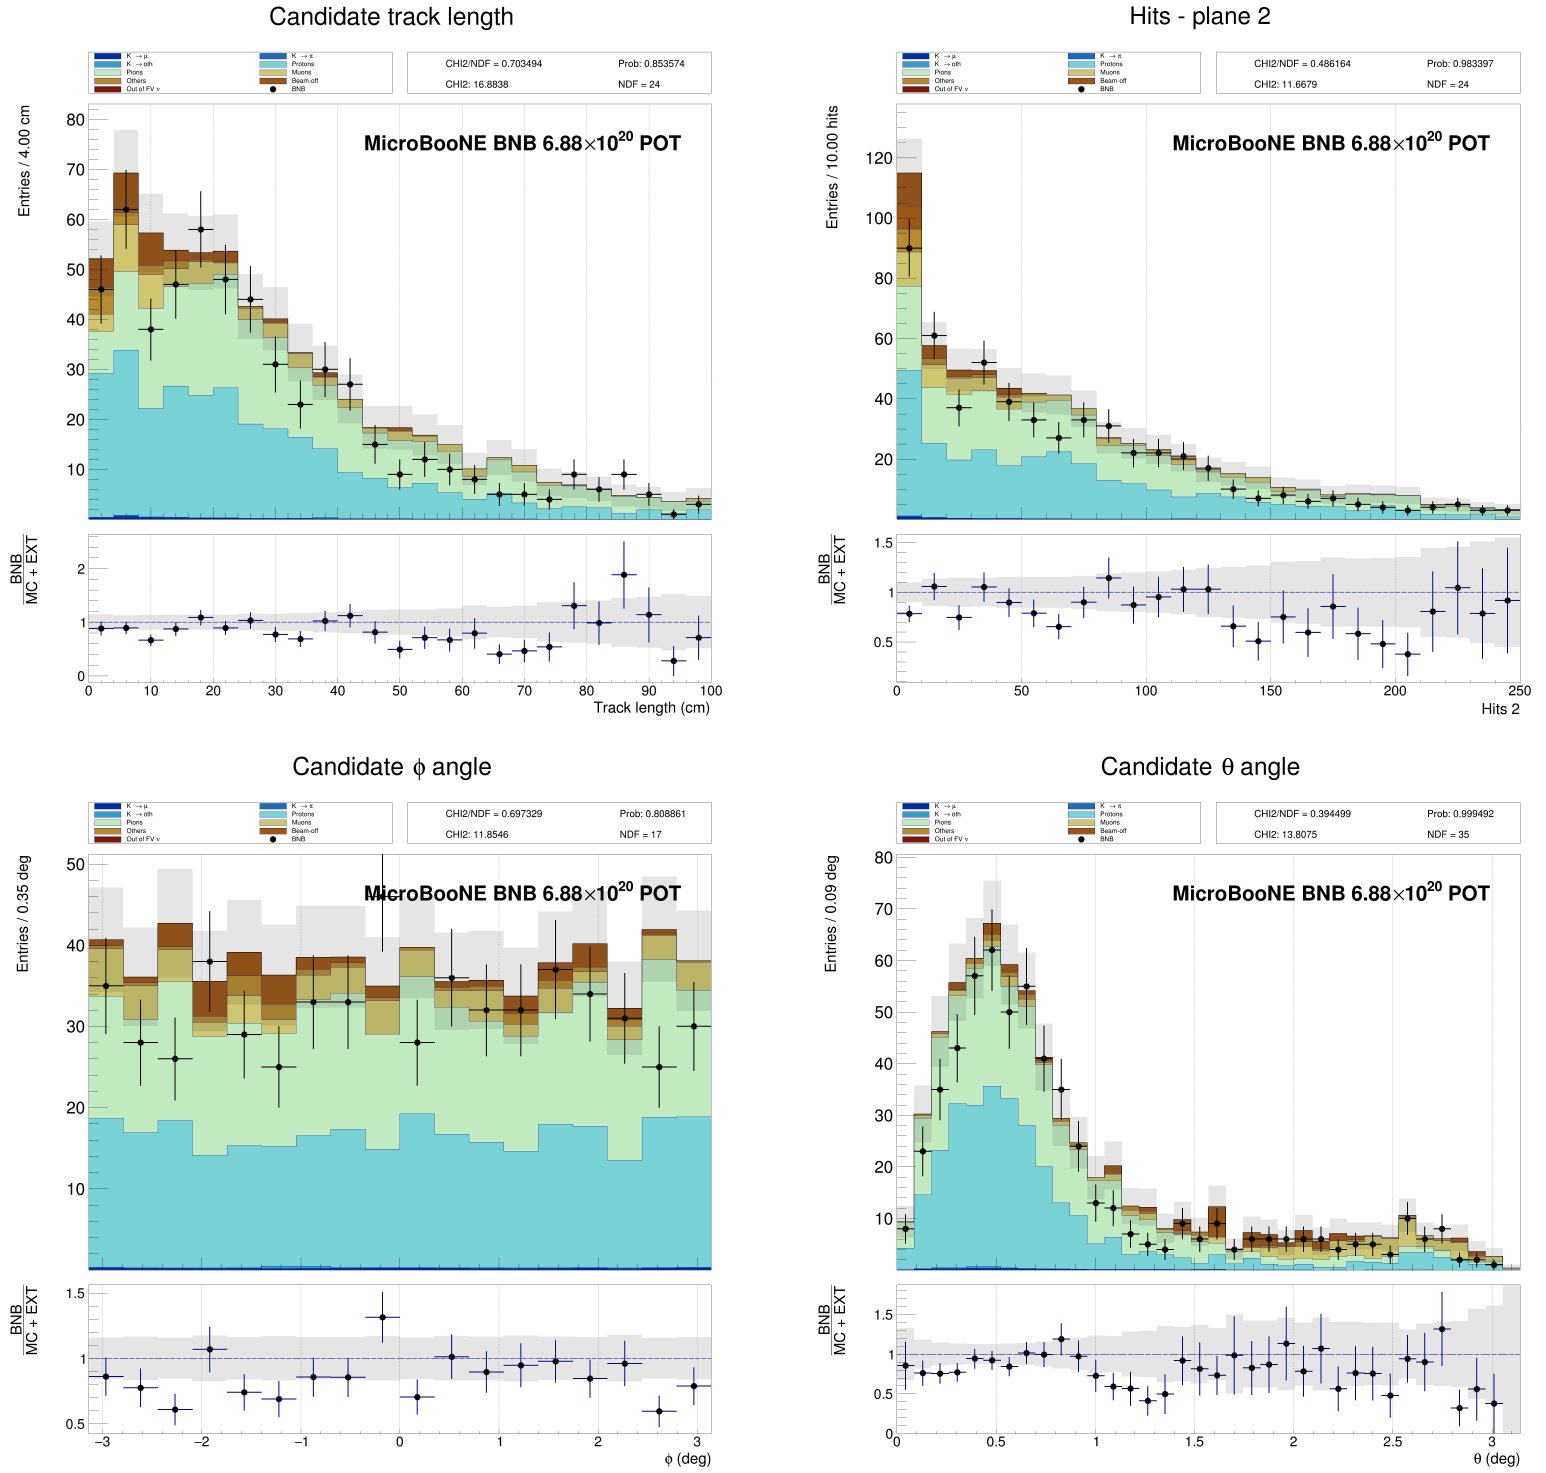

Figure 3: Near sideband data/MC comparisons for track length,  $\phi$ ,  $\theta$  angles, number of hits on collection plane (plane 2).

## II. EVENT DISPLAY OF EVENTS SELECTED IN DATA RUN 1-3

This section shows the event displays of the 10 selected kaon candidates in the  $6.88 \times 10^{20}$  POT dataset used for this analysis. For each panel below (Figures 4 and 5), the event displays were generated from the TPC collection plane view.

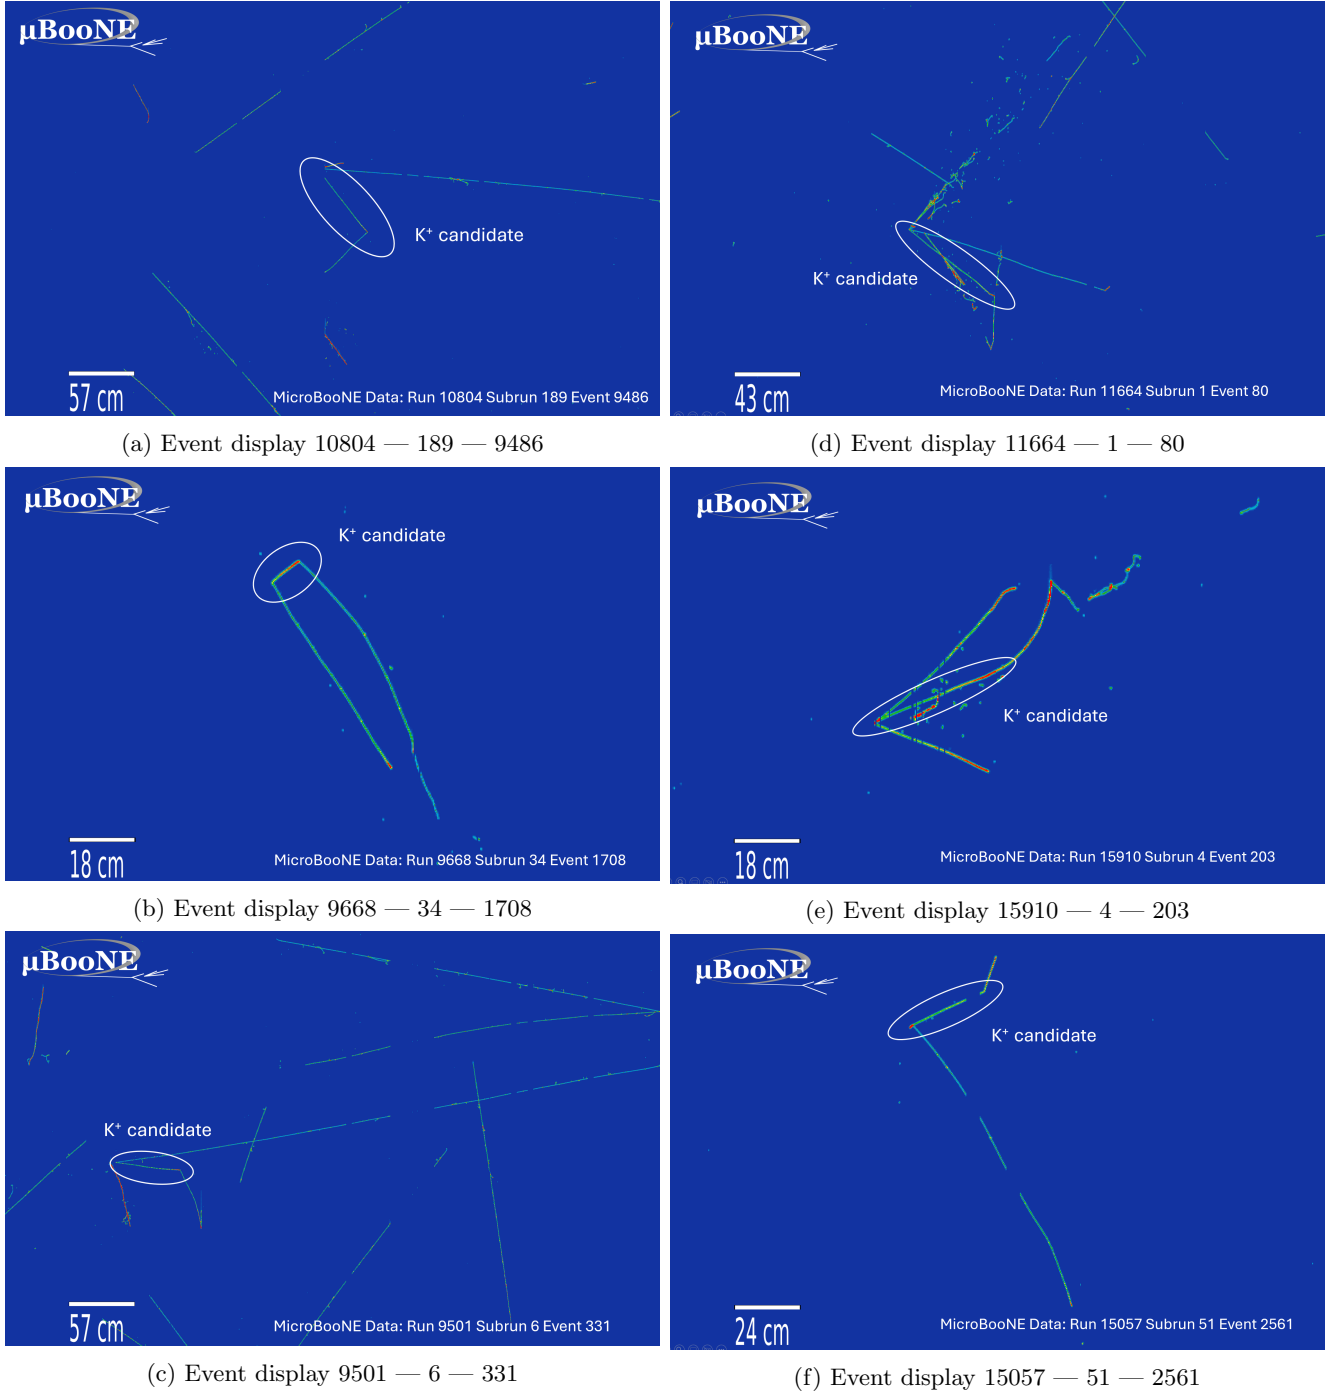

Figure 4: Event display of  $K^+$  candidates.

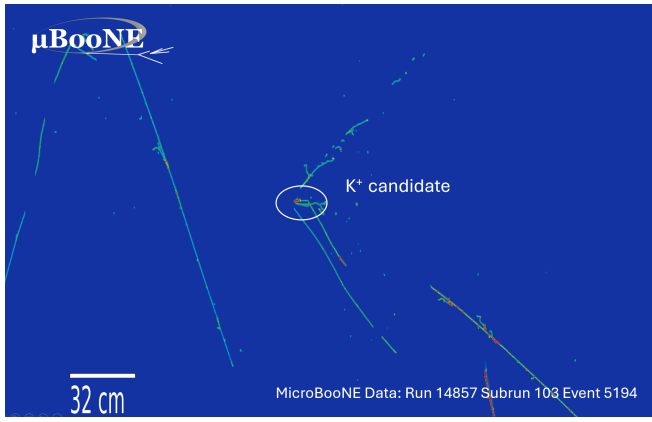

(a) Event display 14857 — 103 — 5194

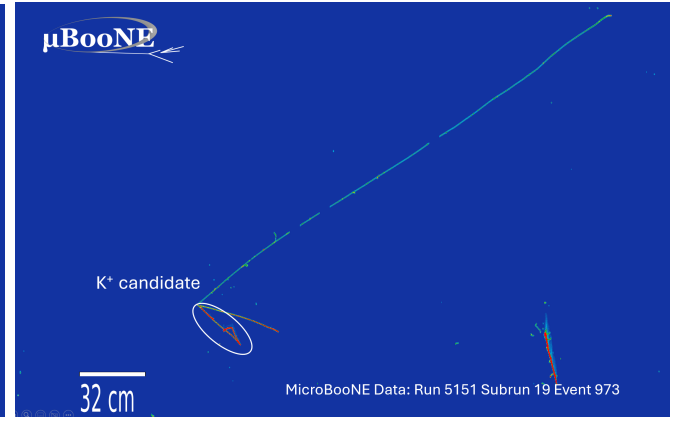

(c) Event display 5151 — 19 — 973

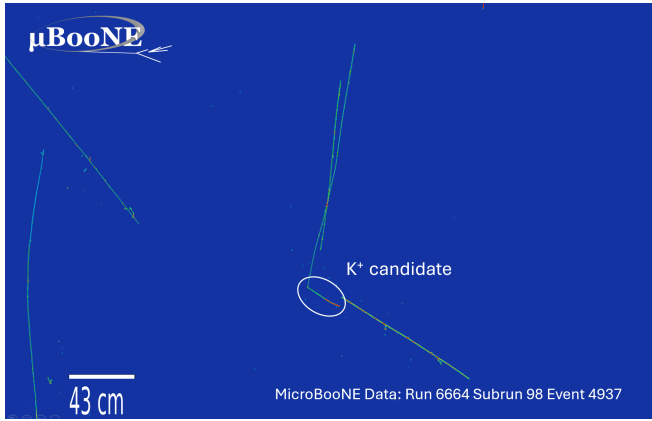

(b) Event display 6664 — 98 — 4937

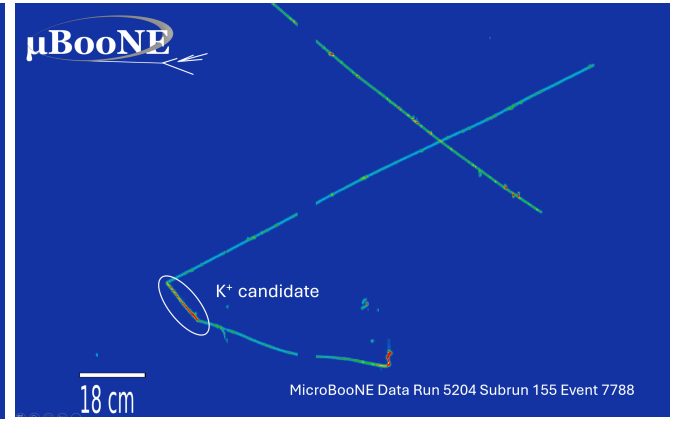

(d) Event display 5204 — 155 — 7788

Figure 5: Event display of  $K^+$  candidates.

### III. EXPECTED BACKGROUND FROM MC IN THE SIGNAL REGION (BDT > 0.41)

This section shows a background event in the signal region. Backgrounds are mainly protons that have attached tracks at their endpoint that mimic a  $K^+$  decay products. Fig. 6 shows an example of an event display of a background event selected in the signal region in the MC BNB sample.

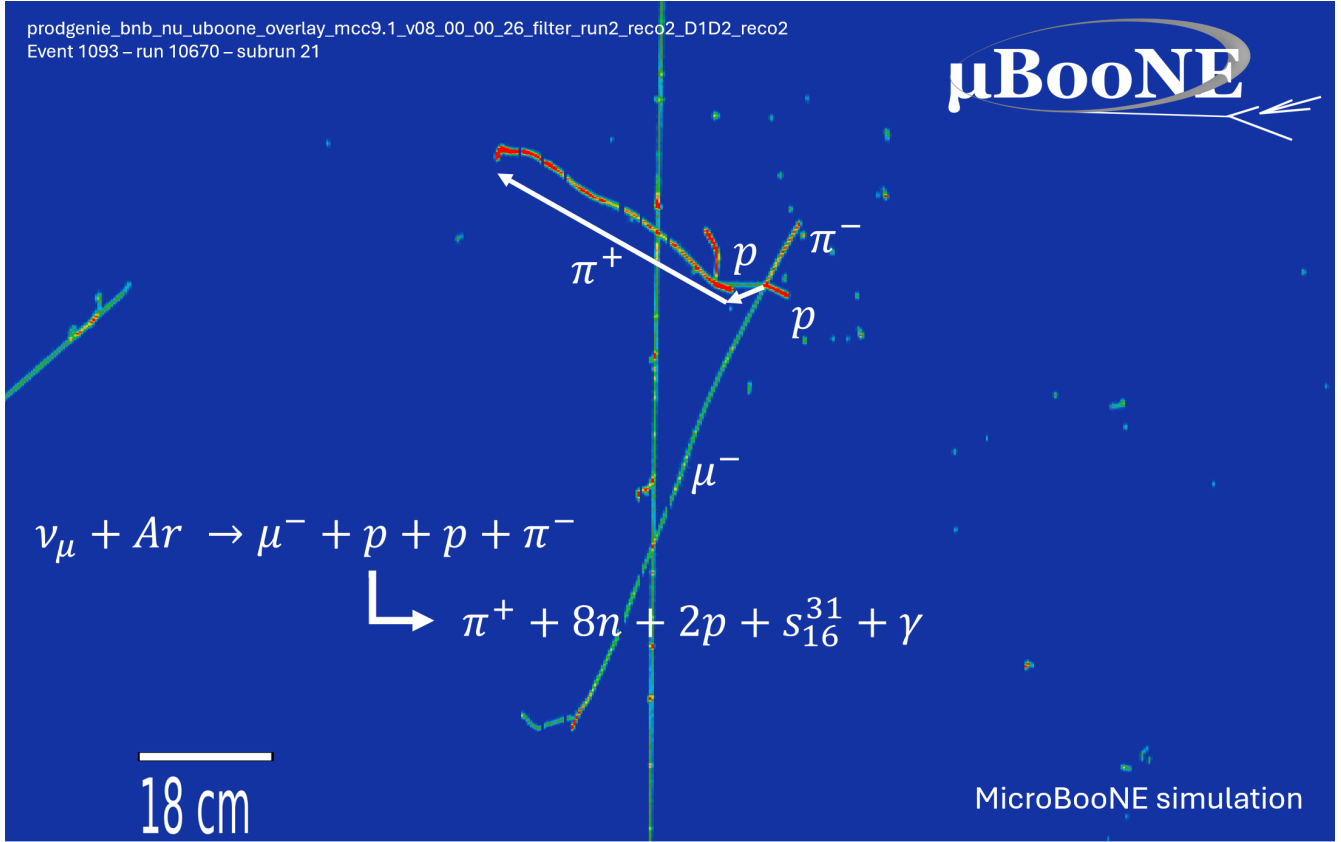

Figure 6: Background event selected in the signal region (BDT > 0.41).

#### IV. DATA AND GEANT4 CROSS-SECTION IN $K^+ - \text{Ca}$ INTERACTIONS

In this section, we compare data with the GEANT4 cross-section for  $K^+ - \text{Ca}$  interactions. A 40% discrepancy between the available  $K^+ - \text{Ca}$  data and the GEANT4 model is observed. We use this to conservatively estimate the  $K^+ - \text{Ar}$  reinteraction uncertainty as  $\pm 40\%$ .

Figure 7 shows the  $K^+ - \text{Ca}$  interaction's data [1] (black triangles), the red curve is the GEANT4  $K^+ - \text{Ca}$  cross-section as a function of the kinetic energy of the  $K^+$ , and green curves represent  $\pm 40\%$  variation on the  $K^+$  inelastic cross-section component to cover the  $K^+ - \text{Ca}$  data in low energy region.

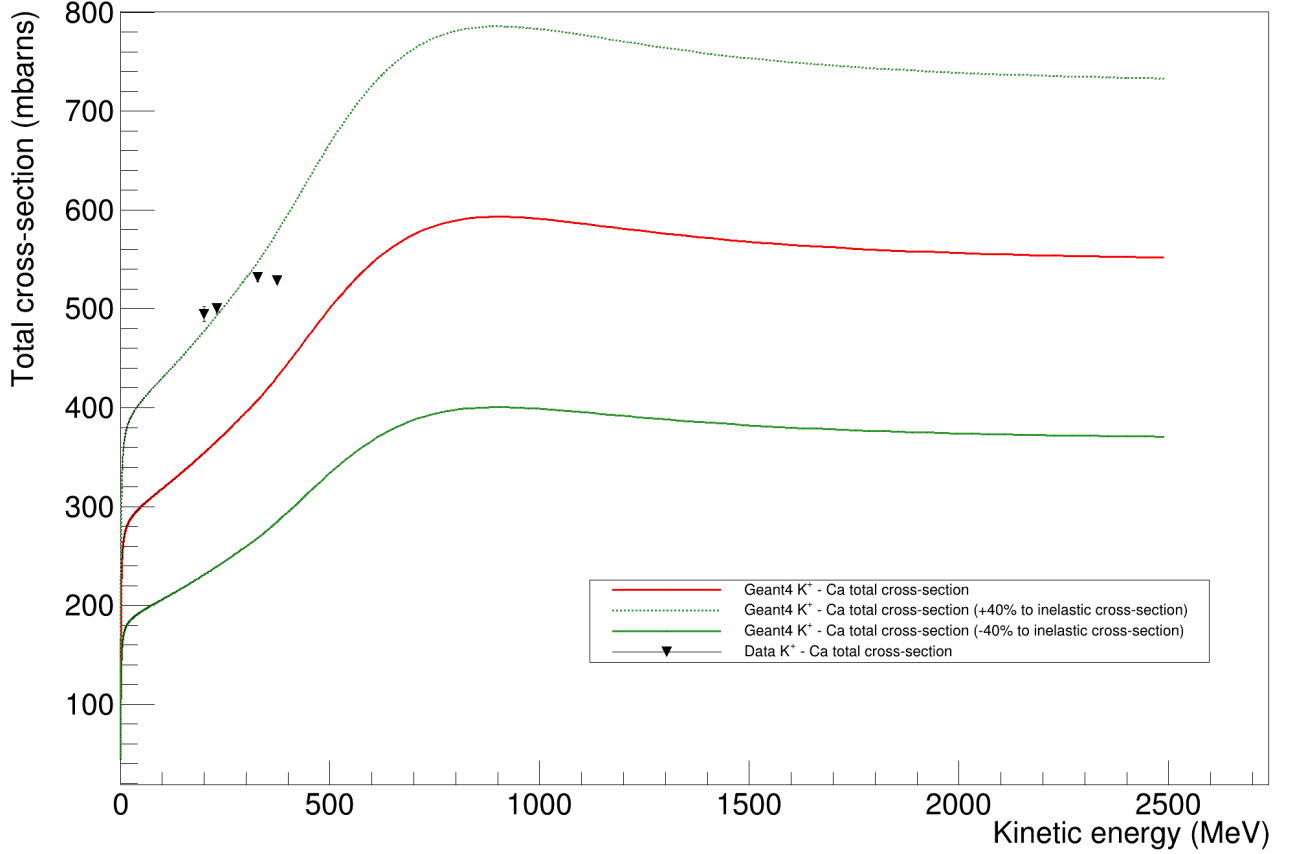

Figure 7: Data and GEANT4 cross-section in  $K^+ - \text{Ca}$  interactions. Green curves represent a plus (dashed green line) and minus (green line) 40 percent variation of the  $K^+ - \text{Ca}$  cross section.

## V. PHASE SPACE CONSTRAINT FOR CHARGED-CURRENT $K^+$ PRODUCTION CROSS-SECTION

This section discusses the phase space constraints applied in this analysis. The identification of a region where  $K^+$  can successfully be reconstructed was done by evaluating the efficiency of reconstructed tracks for signal events as a function of  $K^+$  momentum. The efficiency is defined as the ratio of reconstructed  $K^+$ , with attached daughter tracks at the  $K^+$  endpoint and contained within the fiducial volume, to the total number of generated  $K^+$ . It was found that the efficiency drops to zero below 230 MeV and above 2900 MeV, establishing these values as the phase space constraints for this analysis.

Figure 8 shows the final cross-section calculated with the MicroBooNE dataset analyzed and reported in Table 1 of the letter.

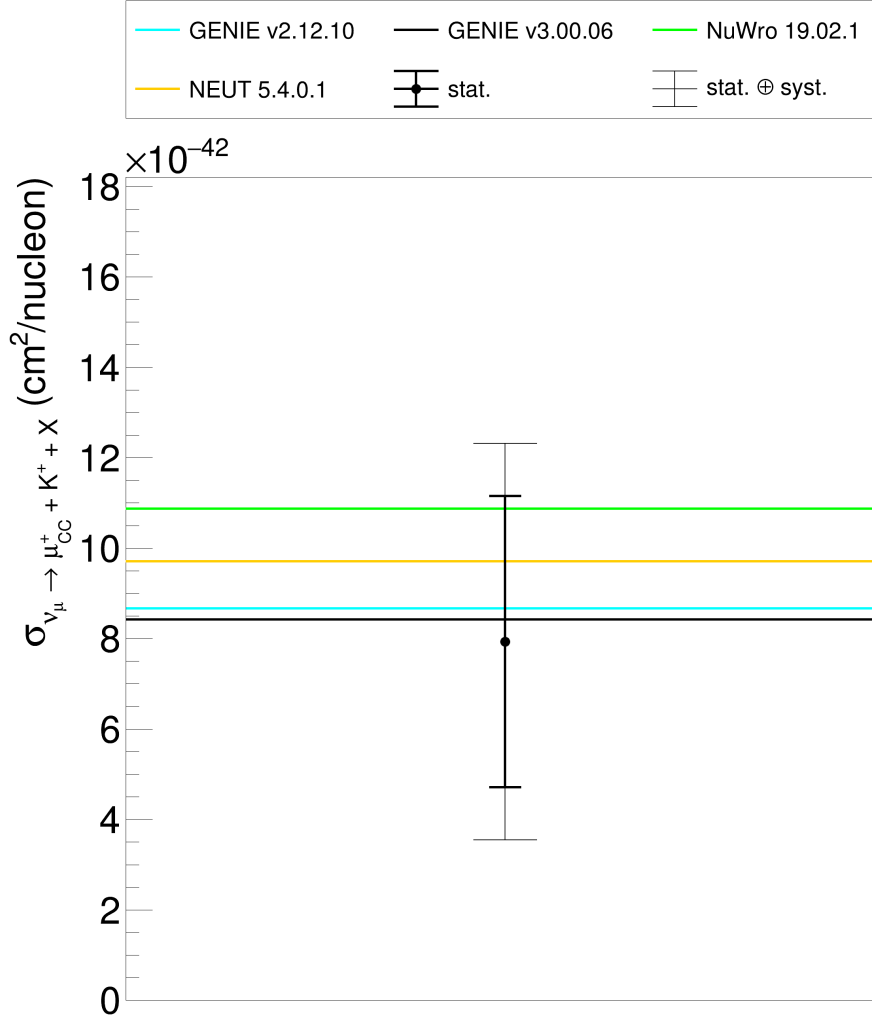

Figure 8: Cross-section calculated after applying the phase space constraint. The black dot represents the measurement in data. Color lines are the cross-section expected from other neutrino generators, where the phase space constraint was also applied.

- 
- [1] R. Weiss *et al.*, “Measurement of low energy  $K^+$  total cross sections on N=Z nuclei,” *Phys. Rev. C*, vol. 49, pp. 2569–2577, May 1994.
